# Supplementary material for: Precision Determination of the Neutral Weak Form Factor of $^{48}$Ca
Source: arXiv:2205.11593 ancillary file (2022-06-16)
Supplement: Supplementary file 1 [file Supplemental_Material.pdf]

# Supplementary Material: Precision Determination of the Neutral Weak Form Factor of $^{48}\text{Ca}$

(The CREX Collaboration)  
(Dated: June 16, 2022)

In this supplementary material we provide a number of important details for the CREX experiment.

## Contents

|                                                                    |   |
|--------------------------------------------------------------------|---|
| I. Acceptance Function                                             | 1 |
| II. Ground State Charge Density of $^{48}\text{Ca}$                | 1 |
| III. Weak Charge of $^{48}\text{Ca}$                               | 2 |
| IV. Parity violating asymmetry from $^{40}\text{Ca}$               | 2 |
| V. Inelastic Contributions                                         | 2 |
| A. Fraction of accepted rate from inelastic scattering             | 3 |
| B. Parity violating asymmetry of excited states                    | 3 |
| 1. Neutron to proton ratio from hadronic scattering                | 3 |
| 2. Random phase approximation calculations                         | 3 |
| 3. Schematic core polarization calculations                        | 4 |
| VI. Relativistic and Non-relativistic Density Functional Models    | 4 |
| VII. Model error for neutron skin of $^{208}\text{Pb}$ from PREX-2 | 6 |
| References                                                         | 6 |

## I. Acceptance Function

The relative acceptance as a function of the lab-frame polar scattering angle is described by the acceptance function  $\epsilon(\theta)$ . This function is constrained to match the observed distributions of the scattered momentum and angle and is generated through Monte Carlo simulation. Important factors accounted for in the simulation include the initial and final state radiation, energy loss, multiple scattering within the target, as well as the geometric acceptance and spectrometer magnetic fields. A family of simulation models are used to reproduce the observed scattering angle  $\langle\theta_{\text{lab}}\rangle_{\text{obs}}$  and 4-momentum transfer squared  $\langle Q^2 \rangle_{\text{obs}}$ .

The range of variation in calculated  $\langle A_{PV} \rangle$  for these simulation models determines the uncertainty ascribed to the acceptance function. The  $A_{PV}$  calculations are performed using both the FSUGold nuclear model [1] and a second model based on a two-parameter Fermi function model for  $\rho_W$ , with common theoretical estimates for the radius and surface thickness. The quoted uncertainty also incorporates the accuracy of the spectrometer

optics calibration which determined the absolute angle to a precision of  $0.02^\circ$ .

The acceptance function  $\epsilon(\theta)$  is shown in Fig. 1 in 100 bins, from  $3^\circ$  to  $8^\circ$ , and arbitrarily normalized to sum to unity over the full acceptance:

$$\sum_i \epsilon(\theta_i) \sin(\theta_i) \Delta\theta = 1 \quad (1)$$

with  $\Delta\theta = 0.05^\circ$ . The acceptance function is provided in a separate file (CREX\_Acceptance.txt) in the supplementary information.

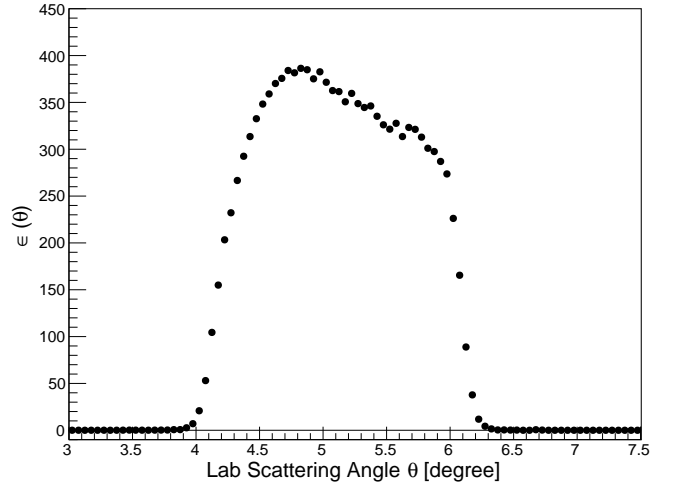

FIG. 1. Acceptance function  $\epsilon(\theta)$  for the CREX measurement.

## II. Ground State Charge Density of $^{48}\text{Ca}$

The ground state charge density of  $^{48}\text{Ca}$ ,  $\rho_{\text{ch}}(r)$ , has been determined by Emrich et al. [2] from electron scattering at Mainz and Saclay. To parameterize  $\rho_{\text{ch}}(r)$  we start from the accurate sum of Gaussians (SOG) expansion for the charge density of  $^{40}\text{Ca}$  [3] and then add a Fourier Bessel (FB) expansion [4] of the difference in charge densities of  $^{48}\text{Ca}$  and  $^{40}\text{Ca}$ ,

$$\rho_{\text{ch}}(r) = \rho_{40}^{\text{SOG}}(r) + \rho_{48}^{\text{FB}}(r) - \rho_{40}^{\text{FB}}(r). \quad (2)$$

This procedure reproduces the electron scattering data and yields a more accurate charge radius than just using  $\rho_{48}^{\text{FB}}(r)$  alone (see Table I). The charge densities are plotted in Fig. 2 and coefficients for the different expansions are from ref. [5].

TABLE I. Elastic charge density parameterizations for  $^{48}\text{Ca}$  with RMS charge radius  $R_{\text{ch}}$  and charge form factor  $F_{\text{ch}}$ . We evaluate the form factor at  $q = 0.8733 \text{ fm}^{-1}$ . We also include the theoretical charge density predicted by the FSUGold relativistic mean field interaction.

| Method                                        | $R_{\text{ch}}$ [fm] | $F_{\text{ch}}(Q^2)$ |
|-----------------------------------------------|----------------------|----------------------|
| FSUGold                                       | 3.4709               | 0.1585               |
| Fourier-Bessel ( $\rho_{48}^{\text{FB}}$ )    | 3.4512               | 0.1574               |
| Sum of Gaussians ( $\rho_{48}^{\text{SOG}}$ ) | 3.4601               | 0.1587               |
| Mixed [Eq. 2]                                 | 3.4807               | 0.1581               |
| Experiment [6]                                | 3.4776               | -                    |

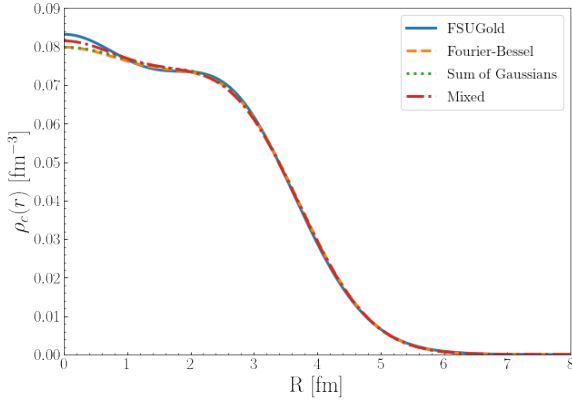

FIG. 2. Experimental charge densities of  $^{48}\text{Ca}$  detailed in the text. We also include the relativistic interaction FSUGold's prediction as a reference point.

### III. Weak Charge of $^{48}\text{Ca}$

The weak charge of a nucleus with  $Z$  protons and  $N$  neutrons is approximately,

$$Q_W = Zq_p + Nq_n, \quad (3)$$

where  $q_p$  is the proton and  $q_n$  the neutron weak charge. Using the Standard model predictions of  $q_p = 0.0711 \pm 0.0002$  and  $Q_W(^{133}\text{Cs}) = -73.23 \pm 0.01$  for Cs atomic parity violation [7] and Eq. 3 gives  $q_n = -0.9890 \pm 0.0002$  and  $Q_W(^{48}\text{Ca}) = -26.27 \pm 0.01$ . However, the  $\gamma - Z$  box radiative correction [8] depends on experimental kinematics and is somewhat different for this measurement compared to Cs atomic parity experiment. Correcting the  $\gamma - Z$  box for the present kinematics yields [9],

$$Q_W(^{48}\text{Ca}) = -26.0 \pm 0.1, \quad (4)$$

which is the value we use.

### IV. Parity violating asymmetry from $^{40}\text{Ca}$

The  $N = Z$  nucleus  $^{40}\text{Ca}$  is expected to have nearly equal proton and neutron densities. We calculate the

weak form factor of  $^{40}\text{Ca}$  as follows,

$$F_W(q) = F_W^{\text{mod}}(q) - F_{\text{ch}}^{\text{mod}}(q) + F_{\text{ch}}^{\text{exp}}(q), \quad (5)$$

using  $Q_W = -18.2$ . Here  $F_W^{\text{mod}}$  and  $F_{\text{ch}}^{\text{mod}}$  are calculated from a series of density functional models and  $F_{\text{ch}}^{\text{exp}}$  is calculated from the experimental charge density of  $^{40}\text{Ca}$  [3]. This procedure minimizes sensitivity to errors in  $F_{\text{ch}}^{\text{mod}}$ . The difference  $F_W^{\text{mod}} - F_{\text{ch}}^{\text{mod}}$  is small and nearly insensitive to the model used. We then Fourier transform  $F_W$  from Eq. 5 to get  $\rho_W(r)$  and calculate  $A_{\text{PV}}$  including Coulomb distortions from the experimental charge density [3] and an integration over acceptance, see Table II. We obtain,

$$A_{\text{PV}}(^{40}\text{Ca}) = 2430 \pm 30 \text{ ppb}, \quad (6)$$

for the  $^{40}\text{Ca}$  correction where the conservative  $\pm 30$  ppb uncertainty includes a contribution from radiative corrections.

TABLE II. Parity violating asymmetry of  $^{40}\text{Ca}$  averaged over acceptance as calculated for different models.

| Model      | $A_{\text{PV}}$ [ppb] |
|------------|-----------------------|
| FSUGold[1] | 2430                  |
| NL3[10]    | 2429                  |
| SI[11]     | 2423                  |

### V. Inelastic Contributions

The electron flux accepted by the integrating quartz detector included contributions from scattering from nuclear excited states. Existing electron scattering data [12, 13] indicate three low-lying excited states of  $^{48}\text{Ca}$  with potentially non-negligible contributions: 3.831 MeV ( $2^+$ ), 4.507 MeV ( $3^-$ ), and 5.370 MeV ( $3^-$ ). Table III lists, for each of these states, the measured yield, the theoretical  $A_{\text{PV}}$  predicted and the resulting correction and uncertainty adopted in Table I of the main paper. The correction for the 4.507 MeV state is small because the  $A_{\text{PV}}^{\text{inel}}$  is close to that of the measured elastic  $A_{\text{PV}}$  for  $^{48}\text{Ca}$ . These numbers are justified in the following discussion.

TABLE III. Experimental Yields, theoretical asymmetries and adopted corrections for  $^{48}\text{Ca}$  low lying excited states.

| State                    | Yield %         | $A_{\text{PV}}^{\text{inel}}$ [ppm] | Correction [ppb] |
|--------------------------|-----------------|-------------------------------------|------------------|
| $2^+(3.831 \text{ MeV})$ | $0.59 \pm 0.12$ | $8.1 \pm 2.7$                       | $-35 \pm 19$     |
| $3^-(4.507 \text{ MeV})$ | $0.66 \pm 0.13$ | $2.7 \pm 1.4$                       | $0 \pm 10$       |
| $3^-(5.370 \text{ MeV})$ | $0.12 \pm 0.02$ | $3.8 \pm 2.7$                       | $-2 \pm 4$       |

### A. Fraction of accepted rate from inelastic scattering

The momentum spectrum of scattered electrons was measured using reduced beam current on the production target to allow momentum and scattering angle reconstruction of individual tracked electrons. The top panel in Fig. 3 shows the spectrum in the spectrometer (black line), along with the spectrum accepted by the integrating detectors (shaded red). The ratio of these curves is the acceptance as a function of momentum and is shown in the bottom panel.

A combined fit of the momentum spectrum was performed which included scattering peaks from the ground state, the three inelastic levels, and the radiative tail. The instrumental resolution of about 310 keV is assumed to be the same for each peak, but the inelastic excitation energy and intensities were independently fit. The fit reproduced the observed spectrum, and the implied relative cross-sections were found to be consistent with existing data. The resulting accepted fraction for each state is listed in Table IV. In total, inelastically scattered electrons contributed 1.4% of the accepted rate. A conservative fractional uncertainty of 20% was applied to the background fraction for each inelastic state.

TABLE IV. Fraction of the total accepted rate from each inelastic level.

| Nuclear State and Excitation | Rate Fraction       |
|------------------------------|---------------------|
| $2^+$ (3.831 MeV)            | $0.59\% \pm 0.12\%$ |
| $3^-$ (4.507 MeV)            | $0.66\% \pm 0.13\%$ |
| $3^-$ (5.370 MeV)            | $0.12\% \pm 0.02\%$ |

### B. Parity violating asymmetry of excited states

We approximate the parity violating asymmetry for inelastic excitations as,

$$A_{PV} \approx \frac{G_F Q^2}{4\pi\alpha\sqrt{2}} \frac{F_t^n(q)}{F_t^p(q)}. \quad (7)$$

Here  $F_t^n$  ( $F_t^p$ ) is the neutron (proton) transition form factor. This is the Fourier transform of the overlap of the ground and excited state wave functions with the density operator. We neglect Coulomb distortions, transverse currents, single nucleon form factors and the weak charge of the proton. The most important nuclear structure input is the ratio of neutron to proton transition form factor  $R_{n/p} = F_t^n/F_t^p$ . We estimate this ratio with (1) phenomenological relations based on hadronic scattering data, (2) non-relativistic and relativistic random phase approximation (RPA) calculations, and (3) a simple core polarization model.

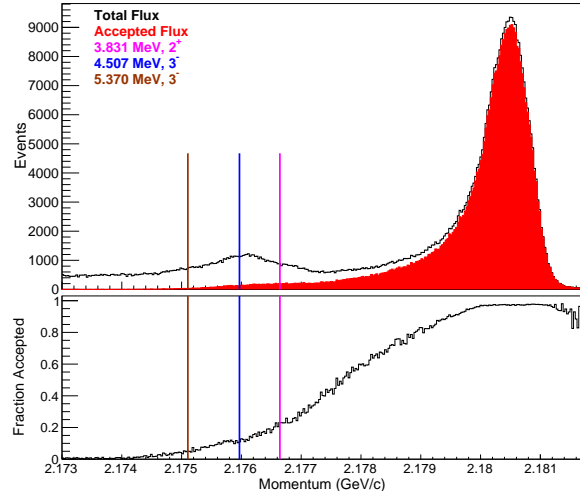

FIG. 3. Momentum spectrum in the spectrometer (top) and acceptance as a function of momentum in the spectrometer (bottom). The significant inelastic levels are marked. Shaded region in the momentum spectrum registered pulses in the integrating detector.

### 1. Neutron to proton ratio from hadronic scattering

The cross section for inelastic electron scattering determines the proton transition density [12]. The neutron transition density can be determined phenomenologically from alpha, proton, or neutron scattering data. For the  $2^+$  (3.831 MeV) state alpha scattering suggests  $R_{n/p}$  is large [14], see Table V. This large ratio is confirmed with neutron scattering data [15].

TABLE V. Ratio of neutron to proton transition form factors  $R_{n/p} = F_t^n/F_t^p$  and parity-violating asymmetry  $A_{PV}$ , see Eq. 7, for the  $2^+$  (3.831 MeV) state in  $^{48}\text{Ca}$  using the different methods described in the text.

| Method                      | $R_{n/p}$ | $A_{PV}$ [ppm] |
|-----------------------------|-----------|----------------|
| Schematic core polarization | 3.3       | 8.8            |
| Non-relativistic RPA [16]   | 2.05      | 5.5            |
| Relativistic RPA [17]       | 2.03      | 5.4            |
| $\alpha$ -Scattering [14]   | 3.2       | 8.5            |
| n-Scattering [15]           | 3.8       | 10.0           |

### 2. Random phase approximation calculations

Random phase approximation (RPA) calculations have been performed for the  $2^+$  (3.831 MeV) state using non-relativistic Skyrme [16] and relativistic mean field residual interactions [17]. These calculations yield proton and neutron transition form factors plotted in Fig. 4 and  $R_{n/p} \approx 2$  as listed in Table V. Details of these calcu-

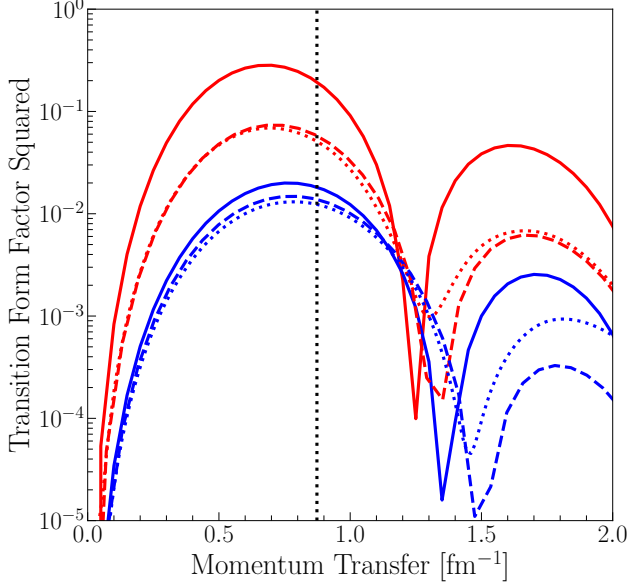

FIG. 4. Transition form factors for the  $2^+$  (3.831 MeV) state in  $^{48}\text{Ca}$ . The three upper red curves show neutron  $|F_t^n|^2$  and the three lower blue curves show proton  $|F_t^p|^2$  transition form factors. The solid, dotted, and dashed lines represent the core polarization, relativistic RPA [17], and non-relativistic RPA [16] calculations respectively. The vertical dashed line shows the momentum transfer of the CREX experiment.

lations will be described in a latter work.

### 3. Schematic core polarization calculations

We now present a very simple core polarization calculation to describe transition form factors. We start with a pure single particle-hole excitation, for example the  $2^+$  state involves a neutron  $1f_{7/2}$  hole and a  $2p_{3/2}$  particle. Following the work of Wise et al. [12], the neutron transition density is

$$\rho_t^{n0} = C_{ab}^\lambda \frac{G_a(r)G_b(r)}{r^2}. \quad (8)$$

Here  $a$  is the hole state ( $1f_{7/2}$ ),  $b$  is the particle ( $2p_{3/2}$ ) and  $\lambda$  is the multipolarity of the transition (2). For simplicity we use the upper components of Dirac wavefunctions for  $G_a(r)$  and  $G_b(r)$  calculated with the FSUGold interaction. The coefficient  $C_{ab}^\lambda$  is [12],

$$C_{ab}^\lambda = (-1)^{\lambda+j_b-1/2} \frac{\hat{j}_a \hat{j}_b}{\sqrt{4\pi}} \langle j_a \frac{1}{2} j_b \frac{-1}{2} | \lambda 0 \rangle \quad (9)$$

with  $\hat{j}_i = \sqrt{2j_i + 1}$ . In this approximation the proton transition density is zero,  $\rho_t^{p0} = 0$ .

We now add a schematic core polarization contribution proportional to  $\epsilon r d\rho/dr$  where  $\rho$  is the ground state

density and  $\epsilon$  is a phenomenological strength to be fit to data. The total neutron transition density is now,

$$\rho_t^n(r) = (1 + \epsilon r \frac{d\rho_n(r)}{dr}) \rho_t^{n0}(r), \quad (10)$$

while the proton transition density has only a core polarization contribution,

$$\rho_t^p(r) = \epsilon r \frac{d\rho_p(r)}{dr} \rho_t^{p0}(r), \quad (11)$$

with  $\rho_n(r)$  the neutron and  $\rho_p(r)$  the proton ground state density. The transition form factors are [12],

$$F_t^i(q^2) = \sqrt{2J+1} \int_0^\infty j_\lambda(qr) \rho_t^i(r) r^2 dr, \quad (12)$$

with  $j_\lambda$  a spherical Bessel function and  $J = 2$  the spin of the excited state. We choose  $\epsilon$  such that  $|F_t^p(q)|^2$  reproduces the measured inelastic electron scattering cross section [12] at  $q = 0.8733 \text{ fm}^{-1}$ , see Table VI. We plot  $|F_t^p(q)|^2$  and  $|F_t^n(q)|^2$  in Fig. 4 where they agree qualitatively with the RPA calculations. The ratio  $R_{n/p} \approx 3.3$  is somewhat larger than RPA predictions and agrees well with that inferred from  $\alpha$  scattering, see Table V. We perform similar calculations for the  $3^-$  (4.507 MeV) and  $3^-$  (5.370 MeV) states.

We show in Table VI the results of this core polarization formalism. We see that the value of  $A_{PV}$  from the  $2^+$  state is the largest of the three with the first  $3^-$  state having the smallest value. Combining these predictions with the results of RPA calculations and hadronic scattering we assign values for the three inelastic states with conservative error bars as listed in Table III.

TABLE VI. Core polarization calculations of excited states.

| Transition        | $ F_t^n ^2$           | $\epsilon [\text{fm}^3]$ | $A_{pv}^{\text{inel}} [\text{ppm}]$ |
|-------------------|-----------------------|--------------------------|-------------------------------------|
| $2^+$ (3.831 MeV) | 0.1934                | -4.366                   | 8.76                                |
| $3^-$ (4.507 MeV) | $1.95 \times 10^{-2}$ | 3.237                    | 1.87                                |
| $3^-$ (5.370 MeV) | $1.49 \times 10^{-2}$ | 4.795                    | 3.44                                |

### VI. Relativistic and Non-relativistic Density Functional Models

We describe the relativistic and non-relativistic density functional models shown in Figs. 2 and 5 of the main paper. We utilize 51 different energy density functionals (EDF) spanning a large range of neutron skins. Of these, 28 models use a relativistic formalism whereas the remaining 23 models are non-relativistic. We provide a complete list of EDFs used in the study in Tables VII and VIII along with their predicted values for the slope of the symmetry energy at saturation  $L$  as well as neutron skins ( $R_n - R_p$ ) and charge minus weak form factors ( $F_{\text{ch}} - F_{\text{W}}$ ) for  $^{48}\text{Ca}$  and  $^{208}\text{Pb}$ .

TABLE VII. List of all relativistic energy density functional (EDF) models used in the CREX analysis. Note there are several FSUGold2 and IU- $\delta$  models with different values of the slope parameter of the symmetry energy  $L$ . Also listed are  $R_n - R_p$  and  $F_{\text{skin}} = F_{\text{ch}} - F_{\text{W}}$  for  $^{48}\text{Ca}$  and  $^{208}\text{Pb}$ .

| Model         | $L$<br>[MeV] | $F_{\text{skin}}^{48}$ | $R_n - R_p^{48}$<br>[fm] | $F_{\text{skin}}^{208}$ | $R_n - R_p^{208}$<br>[fm] |
|---------------|--------------|------------------------|--------------------------|-------------------------|---------------------------|
| FSUGarnet[18] | 50.96        | 0.0439                 | 0.1665                   | 0.0232                  | 0.1614                    |
| FSUGold[1]    | 60.44        | 0.0488                 | 0.1974                   | 0.0300                  | 0.2073                    |
| FSUGold2[19]  | 47.00        | 0.0424                 | 0.1641                   | 0.0217                  | 0.1520                    |
| FSUGold2[19]  | 50.00        | 0.0444                 | 0.1736                   | 0.0243                  | 0.1691                    |
| FSUGold2[19]  | 54.00        | 0.0464                 | 0.1830                   | 0.0270                  | 0.1867                    |
| FSUGold2[19]  | 58.00        | 0.0479                 | 0.1902                   | 0.0291                  | 0.2007                    |
| FSUGold2[19]  | 69.00        | 0.0509                 | 0.2041                   | 0.0334                  | 0.2287                    |
| FSUGold2[19]  | 76.00        | 0.0523                 | 0.2105                   | 0.0355                  | 0.2420                    |
| FSUGold2[19]  | 90.00        | 0.0544                 | 0.2204                   | 0.0387                  | 0.2626                    |
| FSUGold2[19]  | 100.00       | 0.0556                 | 0.2260                   | 0.0405                  | 0.2743                    |
| FSUGold2[20]  | 112.68       | 0.0568                 | 0.2319                   | 0.0424                  | 0.2866                    |
| IUFSU[21]     | 47.21        | 0.0440                 | 0.1731                   | 0.0233                  | 0.1618                    |
| NL3[10]       | 118.19       | 0.0555                 | 0.2258                   | 0.0415                  | 0.2802                    |
| RMF022[18]    | 63.52        | 0.0496                 | 0.1967                   | 0.0316                  | 0.2168                    |
| RMF028[18]    | 112.64       | 0.0569                 | 0.2315                   | 0.0422                  | 0.2854                    |
| RMF032[18]    | 125.63       | 0.0587                 | 0.2439                   | 0.0470                  | 0.3206                    |
| TFa[22]       | 82.50        | 0.0529                 | 0.2145                   | 0.0368                  | 0.2505                    |
| TFb[22]       | 122.53       | 0.0569                 | 0.2395                   | 0.0442                  | 0.3006                    |
| TFc[22]       | 135.24       | 0.0583                 | 0.2502                   | 0.0483                  | 0.3313                    |
| IU- $\delta$  | -40.00       | 0.0206                 | 0.0637                   | 0.0043                  | 0.0408                    |
| IU- $\delta$  | -30.00       | 0.0239                 | 0.0795                   | 0.0068                  | 0.0568                    |
| IU- $\delta$  | -20.00       | 0.0271                 | 0.0950                   | 0.0092                  | 0.0722                    |
| IU- $\delta$  | -10.00       | 0.0302                 | 0.1090                   | 0.0123                  | 0.0928                    |
| IU- $\delta$  | 0.00         | 0.0333                 | 0.1234                   | 0.0155                  | 0.1133                    |
| IU- $\delta$  | 10.00        | 0.0359                 | 0.1373                   | 0.0172                  | 0.1247                    |
| IU- $\delta$  | 20.00        | 0.0388                 | 0.1501                   | 0.0202                  | 0.1438                    |
| IU- $\delta$  | 30.00        | 0.0405                 | 0.1589                   | 0.0213                  | 0.1510                    |
| IU- $\delta$  | 40.00        | 0.0442                 | 0.1750                   | 0.0265                  | 0.1846                    |

For the non-relativistic models, we chose the Skyrme EDF and several models which have been popular over the years. These models are chosen so that they span a large range of symmetry energy values as well as properties of finite nuclei. The inclusion of the spin-orbit currents into the calculation of the weak and charge densities is similar to the relativistic case described in [23]. However, we generate the tensor form factors using the wavefunctions of the relativistic FSUGold[1] model in the free-space approximation

$$F(r) \approx \frac{1}{2m} \left( \frac{dG}{dr} + \frac{\kappa}{r} G \right) \quad (13)$$

where  $G(r)$  and  $F(r)$  are the upper and lower components of the Dirac wavefunction respectively. By assuming this free-space relation, we use the expression in [23] for the tensor form factor of the proton and neutron. We then use the Skyrme model's proton and neutron densities for the baryon form factors and calculate the spin-orbit corrected charge and weak densities.

The relativistic models follow the Lagrangian parameterization used by [31] with some including the addition of the spin-zero isovector delta meson. We include the

TABLE VIII. List of all non-relativistic EDF models used in the CREX analysis.

| Model        | $L$<br>[MeV] | $F_{\text{skin}}^{48}$ | $R_n - R_p^{48}$<br>[fm] | $F_{\text{skin}}^{208}$ | $R_n - R_p^{208}$<br>[fm] |
|--------------|--------------|------------------------|--------------------------|-------------------------|---------------------------|
| SI[11]       | 1.22         | 0.0319                 | 0.1216                   | 0.0159                  | 0.1138                    |
| SII[24]      | 9.91         | 0.0345                 | 0.1374                   | 0.0174                  | 0.1246                    |
| SKM*[25]     | 45.76        | 0.0392                 | 0.1551                   | 0.0247                  | 0.1688                    |
| SLy4[26]     | 45.96        | 0.0391                 | 0.1535                   | 0.0234                  | 0.1596                    |
| SLy5[26]     | 48.14        | 0.0403                 | 0.1608                   | 0.0239                  | 0.1622                    |
| SLy7[26]     | 47.22        | 0.0394                 | 0.1598                   | 0.0231                  | 0.1583                    |
| SV-K218[27]  | 34.62        | 0.0381                 | 0.1725                   | 0.0231                  | 0.1622                    |
| SV-K226[27]  | 34.09        | 0.0379                 | 0.1693                   | 0.0228                  | 0.1599                    |
| SV-K241[27]  | 30.95        | 0.0379                 | 0.1617                   | 0.0219                  | 0.1527                    |
| SV-bas[27]   | 32.36        | 0.0379                 | 0.1651                   | 0.0223                  | 0.1559                    |
| SV-kap00[27] | 39.44        | 0.0368                 | 0.1627                   | 0.0226                  | 0.1580                    |
| SV-kap02[27] | 35.54        | 0.0373                 | 0.1635                   | 0.0224                  | 0.1565                    |
| SV-kap06[27] | 29.33        | 0.0384                 | 0.1669                   | 0.0222                  | 0.1555                    |
| SV-mas07[27] | 52.15        | 0.0389                 | 0.1764                   | 0.0245                  | 0.1708                    |
| SV-mas08[27] | 40.15        | 0.0383                 | 0.1694                   | 0.0232                  | 0.1616                    |
| SV-mas10[27] | 28.03        | 0.0375                 | 0.1633                   | 0.0219                  | 0.1536                    |
| SV-sym28[27] | 7.21         | 0.0330                 | 0.1444                   | 0.0162                  | 0.1178                    |
| SV-sym32[27] | 57.07        | 0.0421                 | 0.1864                   | 0.0281                  | 0.1933                    |
| SV-sym34[27] | 80.95        | 0.0455                 | 0.2063                   | 0.0335                  | 0.2287                    |
| SV-Min[27]   | 44.81        | 0.0384                 | 0.1739                   | 0.0246                  | 0.1716                    |
| TOV-Min[28]  | 76.23        | 0.0402                 | 0.1900                   | 0.0298                  | 0.2064                    |
| UNEDF0[29]   | 45.08        | 0.0445                 | 0.2104                   | 0.0267                  | 0.1882                    |
| UNEDF1[30]   | 40.00        | 0.0360                 | 0.1845                   | 0.0245                  | 0.1770                    |

delta meson as a simple way to reduce the slope of the symmetry energy, essential in reducing the size of the neutron skin. The delta meson couples to the nucleons via the interaction Lagrangian

$$\mathcal{L}_{\text{int}} = \dots + \bar{\psi} \left( \frac{g_\delta}{2} \tau_3 \delta \right) \psi \quad (14)$$

where  $g_\delta$  is the coupling constant,  $\tau_3$  is an isospin matrix, and  $\delta$  is the neutral meson mean-field.

The generation of new models with the delta meson were performed following a similar technique to that described in [20]. We first start with the parameters of the FSUGold2 set and fix the saturation density of nuclear matter  $\rho_0$ , binding energy per nucleon  $E/A$ , incompressibility  $K$ , and effective nucleon mass at saturation  $M_*$ . The quartic vector self-coupling constant  $\zeta$  helps control the behavior of the high density equation of state and its effects on finite nuclei are small, so we fix it also at the FSUGold2 value. This leaves us with four inputs: the symmetry energy at saturation  $J$ , its slope  $L$ , its curvature  $K_{\text{sym}}$ , and the scalar meson mass  $m_s$ .

To probe a wide range of neutron skins, we fix  $L$  at values between [-40,40] MeV in increments of 10 MeV and let  $J$ ,  $K_{\text{sym}}$ , and  $m_s$  vary. We fit these latter three values to the charge radii and binding energies of magic nuclei to achieve an optimal functional that is good for reproducing properties of finite nuclei. We note that the calculation of the charge radius for the fitting procedure includes the effects of spin-orbit currents, see [23]. For more details on each parameter and the inversion of nu-

clear observables to coupling constants, see ref. [20]. Further details describing these new RMF models, dubbed IU- $\delta$  in Table VII, will be discussed in a latter work.

### VII. Model error for neutron skin of $^{208}\text{Pb}$ from PREX-2

The model error in extracting  $R_n - R_p$  for  $^{208}\text{Pb}$  from the PREX-2 measurement is much smaller than for  $^{48}\text{Ca}$ . This is because PREX-2 was run at a lower momentum transfer and because  $^{208}\text{Pb}$  has a smaller surface to volume ratio than  $^{48}\text{Ca}$ . This makes changes in the surface thickness less important. We illustrate this in Fig. 5. This figure can be directly compared to Fig. 4b in the main text and shows a much smaller spread in  $R_n - R_p$  predicted by the models for a given value of  $F_{\text{ch}} - F_{\text{W}}$ .

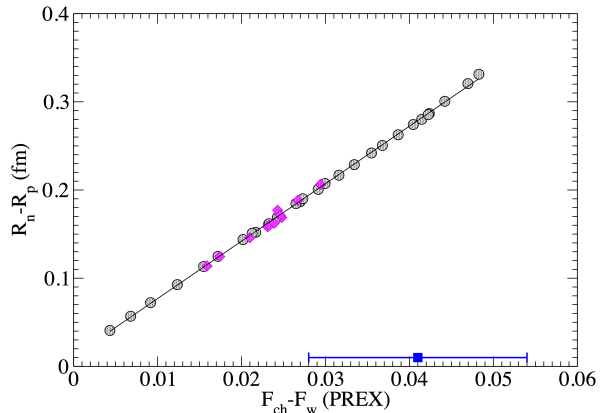

FIG. 5.  $R_n - R_p$  of  $^{208}\text{Pb}$  versus charge minus weak form factor. The blue error bar is the PREX-2 measurement while black circles are relativistic and magenta diamonds are non-relativistic density functional models.

- 
- [1] B. G. Todd-Rutel and J. Piekarewicz, Neutron-Rich Nuclei and Neutron Stars: A New Accurately Calibrated Interaction for the Study of Neutron-Rich Matter, *Phys. Rev. Lett.* **95**, 122501 (2005), arXiv:nucl-th/0504034 [astro-ph].
  - [2] H. J. Emrich, G. Fricke, G. Mallot, H. Miska, H. G. Sieberling, J. M. Cavedon, B. Frois, and D. Goutte, Radial distribution of nucleons in isotopes  $^{48,40}\text{Ca}$ , *Nucl. Phys. A* **396**, 401C (1983).
  - [3] I. Sick, J. Bellicard, J. Cavedon, B. Frois, M. Huet, P. Leconte, P. Ho, and S. Platchkov, Charge density of  $^{40}\text{Ca}$ , *Physics Letters B* **88**, 245 (1979).
  - [4] B. Dreher, J. Friedrich, K. Merle, H. Rothhaas, and G. Lührs, The determination of the nuclear ground state and transition charge density from measured electron scattering data, *Nuclear Physics A* **235**, 219 (1974).
  - [5] H. de Vries, C. W. de Jager, and C. de Vries, Nuclear Charge-Density-Distribution Parameters from Electron Scattering, *Atomic Data and Nuclear Data Tables* **36**, 495 (1987).
  - [6] I. Angeli and K. P. Marinova, Table of experimental nuclear ground state charge radii: an update, *Atomic Data and Nuclear Data Tables* **99**, 69 (2013).
  - [7] P.A. Zyla et al. (Particle Data Group), 2020 review of particle physics, *Prog. Theor. Exp. Phys.* **2020**, 083C01 (2020).
  - [8] M. Gorchtein and C. J. Horowitz, Dispersion  $\gamma$ Z-box correction to the weak charge of the proton, *Phys. Rev. Lett.* **102**, 091806 (2009).
  - [9] Jens Erler and Misha Gorchtein, Private communication (2022).
  - [10] G. A. Lalazissis, J. König, and P. Ring, A new parametrization for the Lagrangian density of relativistic mean field theory, *Phys. Rev. C* **55**, 540 (1997), arXiv:nucl-th/9607039.
  - [11] T. H. R. Skyrme, The effective nuclear potential, *Nuclear Physics* **9**, 615 (1958).
  - [12] J. E. Wise, J. S. McCarthy, R. Altemus, B. E. Norum, R. R. Whitney, J. Heisenberg, J. Dawson, and O. Schwenker, Inelastic electron scattering from  $^{48}\text{Ca}$ , *Phys. Rev. C* **31**, 1699 (1985).
  - [13] R. A. Eisenstein, D. W. Madsen, H. Theissen, L. S. Cardman, and C. K. Bockelman, Electron-Scattering Studies on  $^{40}\text{Ca}$  and  $^{48}\text{Ca}$ , *Phys. Rev.* **188**, 1815 (1969).
  - [14] A. M. Bernstein, V. R. Brown, and V. A. Madsen, Neutron and proton transition matrix elements and inelastic hadron scattering, *Physics Letters B* **103**, 255 (1981).
  - [15] J. R. Vanhoy, M. T. McEllistrem, S. F. Hicks, R. A. Gatenby, E. M. Baum, E. L. Johnson, G. Molnár, and S. W. Yates, Neutron and proton dynamics of  $^{48}\text{Ca}$  levels and  $\gamma$ -ray decays from neutron inelastic scattering, *Phys. Rev. C* **45**, 1628 (1992).
  - [16] P. G. Reinhard and X. Roca-Maza, Private communication (2022).
  - [17] J. Piekarewicz, Private communication (2022).
  - [18] W.-C. Chen and J. Piekarewicz, Searching for isovector signatures in the neutron-rich oxygen and calcium isotopes, *Physics Letters B* **748**, 284 (2015), arXiv:1412.7870 [nucl-th].
  - [19] B. T. Reed, F. J. Fattoyev, C. J. Horowitz, and J. Piekarewicz, Implications of PREX-2 on the equation of state of neutron-rich matter, *Phys. Rev. Lett.* **126**, 172503 (2021), arXiv:2101.03193 [nucl-th].
  - [20] W.-C. Chen and J. Piekarewicz, Building relativistic mean field models for finite nuclei and neutron stars, *Phys. Rev. C* **90**, 044305 (2014), arXiv:1408.4159 [nucl-th].
  - [21] F. Fattoyev, C. Horowitz, J. Piekarewicz, and G. Shen, Relativistic effective interaction for nuclei, giant resonances, and neutron stars, *Phys. Rev. C* **82**, 055803 (2010).

- (2010), arXiv:1008.3030 [nucl-th].
- [22] F. J. Fattoyev and J. Piekarewicz, Has a thick neutron skin in  $^{208}\text{Pb}$  been ruled out?, Phys. Rev. Lett. **111**, 162501 (2013), arXiv:1306.6034 [nucl-th].
  - [23] C. J. Horowitz and J. Piekarewicz, Impact of spin-orbit currents on the electroweak skin of neutron-rich nuclei, Phys. Rev. C **86**, 045503 (2012).
  - [24] D. Vautherin and D. M. Brink, Hartree-Fock Calculations with Skyrme's Interaction. I. Spherical Nuclei, Phys. Rev. C **5**, 626 (1972).
  - [25] J. Bartel, P. Quentin, M. Brack, C. Guet, and H. B. Håkansson, Towards a better parametrisation of Skyrme-like effective forces: A critical study of the SkM force, Nuc. Phys. A **386**, 79 (1982).
  - [26] E. Chabanat, P. Bonche, P. Haensel, J. Meyer, and R. Schaeffer, A Skyrme parametrization from subnuclear to neutron star densities Part II. Nuclei far from stabilities, Nuc. Phys. A **635**, 231 (1998).
  - [27] P. Klüpfel, P. G. Reinhard, T. J. Bürvenich, and J. A. Maruhn, Variations on a theme by Skyrme: A systematic study of adjustments of model parameters, Phys. Rev. C **79**, 034310 (2009).
  - [28] J. Erler, C. J. Horowitz, W. Nazarewicz, M. Rafalski, and P. G. Reinhard, Energy density functional for nuclei and neutron stars, Phys. Rev. C **87**, 044320 (2013), arXiv:1211.6292 [nucl-th].
  - [29] M. Kortelainen, T. Lesinski, J. Moré, W. Nazarewicz, J. Sarich, N. Schunck, M. V. Stoitsov, and S. Wild, Nuclear energy density optimization, Phys. Rev. C **82**, 024313 (2010).
  - [30] M. Kortelainen, J. McDonnell, W. Nazarewicz, P.-G. Reinhard, J. Sarich, N. Schunck, M. V. Stoitsov, and S. M. Wild, Nuclear energy density optimization: Large deformations, Phys. Rev. C **85**, 024304 (2012).
  - [31] C. J. Horowitz and J. Piekarewicz, The neutron radii of Pb-208 and neutron stars, Phys. Rev. C **64**, 062802 (2001), arXiv:nucl-th/0108036.
